# Supplementary material for: Momentum with Variance Reduction for Nonconvex Composition Optimization
Source: arXiv:2005.07755 source file (2020-05-15)
Supplement: Supplementary file 1 [file appendix.tex]

\clearpage
\onecolumn
\appendix
